# Supplementary material for: Structured Learning via Logistic Regression
Source: arXiv:1407.0754 source file (2014-07-03)
Supplement: Supplementary file 1 [file 2013nips_appendix.pdf]

## Appendix for paper: Structured Learning via Logistic Regression

**Theorem 5.** *The difference of  $l$  and  $l_1$  is bounded by*

$$l_1(x, y, F) \leq l(x, y, F) \leq l_1(x, y, F) + \epsilon H_{\max}, \quad H_{\max} = \sum_{\alpha} |y_{\alpha}| \log |y_{\alpha}|.$$

*Proof.* We can write

$$\begin{aligned} l(x, y; F) - l_1(x, y; F) &= -F(x, y) + \max_{\mu \in \mathcal{M}} \left( \theta \cdot \mu + \sum_{\alpha} \epsilon H(\mu_{\alpha}) \right) + F(x, y) - \max_{\mu \in \mathcal{M}} \theta \cdot \mu \\ &= \max_{\mu \in \mathcal{M}} \left( \theta \cdot \mu + \sum_{\alpha} \epsilon H(\mu_{\alpha}) \right) - \max_{\mu \in \mathcal{M}} \theta \cdot \mu \\ &= \theta \cdot \mu' - \theta \cdot \mu^* + \sum_{\alpha} \epsilon H(\mu_{\alpha}) \\ &\leq \epsilon \sum_{\alpha} |y_{\alpha}| \log |y_{\alpha}|. \end{aligned}$$

where, defining  $\mu^* = \arg \max_{\mu \in \mathcal{M}} \theta \cdot \mu$  and  $\mu' = \arg \max_{\mu \in \mathcal{M}} \theta \cdot \mu + \epsilon \sum_{\alpha} H(\mu_{\alpha})$ . The last line follows from the fact that  $\theta \cdot \mu^* \geq \theta \cdot \mu'$ , and that  $H(\mu_{\alpha}) \leq |y_{\alpha}| \log |y_{\alpha}|$ .  $\square$

| Denoising                                  |      |        |        |        |      | Horses                                     |      |        |        |        |      |
|--------------------------------------------|------|--------|--------|--------|------|--------------------------------------------|------|--------|--------|--------|------|
| $\mathcal{F}_i \setminus \mathcal{F}_{ij}$ | Zero | Const. | Linear | Boost. | MLP  | $\mathcal{F}_i \setminus \mathcal{F}_{ij}$ | Zero | Const. | Linear | Boost. | MLP  |
| Zero                                       | .490 | .490   | .490   | .465   | .490 | Zero                                       | .211 | .211   | .212   | .211   | .210 |
| Const.                                     | .490 | .490   | .490   | .465   | .490 | Const.                                     | .211 | .211   | .212   | .211   | .210 |
| Linear                                     | .443 | .077   | .059   | .056   | .033 | Linear                                     | .141 | .139   | .126   | .111   | .113 |
| Boost.                                     | .429 | .032   | .014   | .012   | .008 | Boost.                                     | .087 | .079   | .074   | .069   | .068 |
| MLP                                        | .435 | .031   | .014   | .011   | .008 | MLP                                        | .054 | .051   | .046   | .043   | .041 |

Table 2: Univariate Training Error Rates

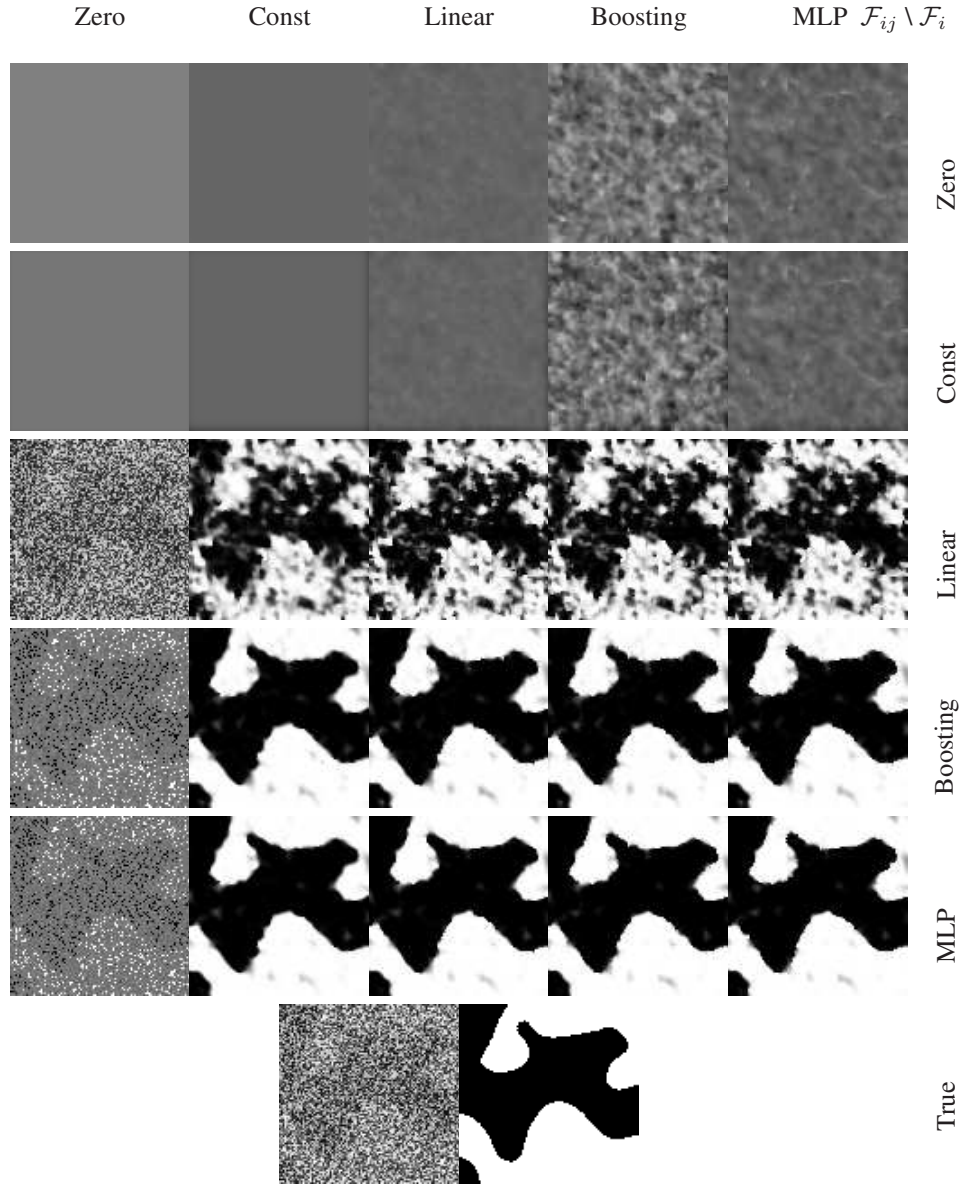

Figure 4: Example Predictions on the Denoising Dataset

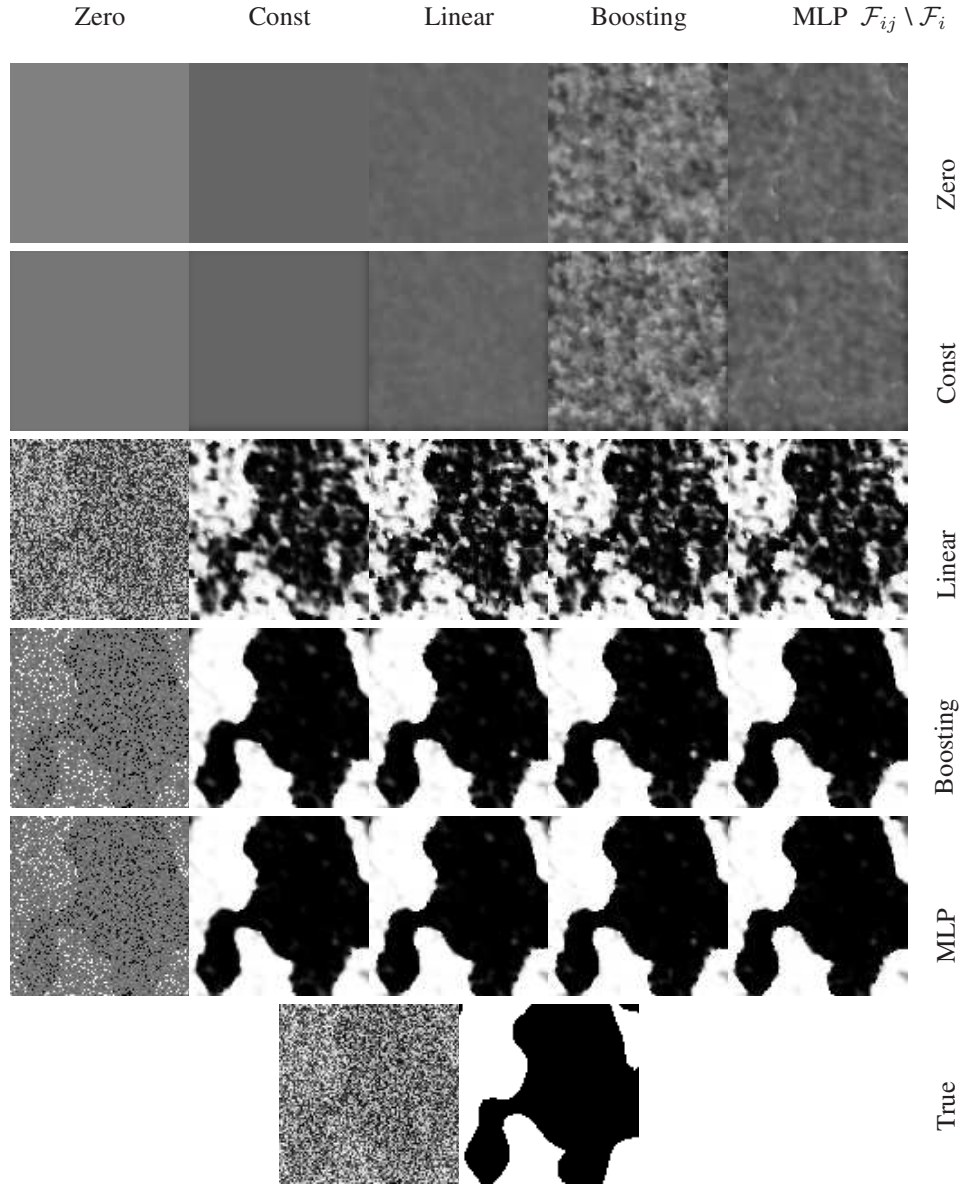

Figure 5: Example Predictions on the Denoising Dataset

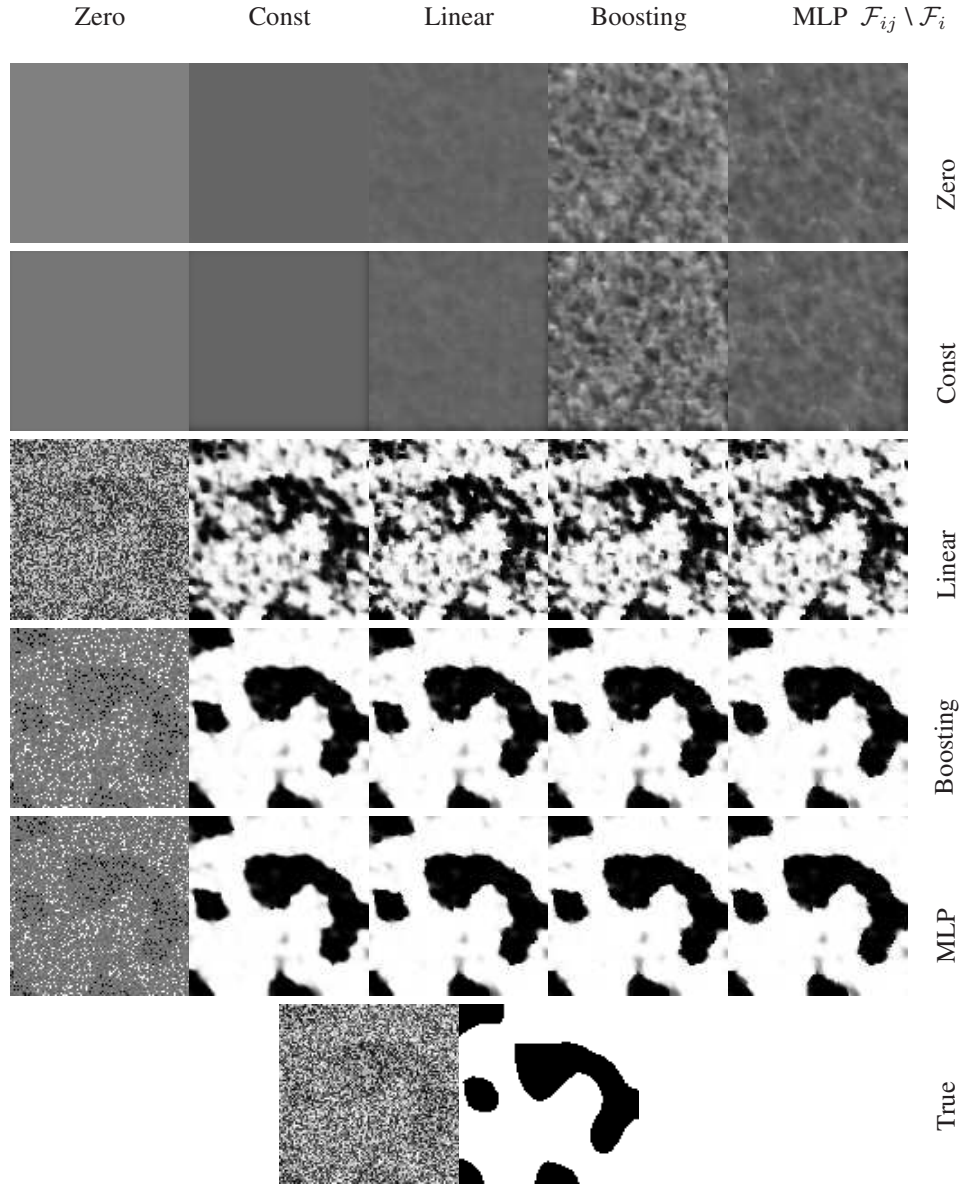

Figure 6: Example Predictions on the Denoising Dataset

702  
703  
704  
705  
706  
707  
708  
709  
710  
711  
712  
713  
714  
715  
716  
717  
718  
719  
720  
721  
722  
723  
724  
725  
726  
727  
728  
729  
730  
731  
732  
733  
734  
735  
736  
737  
738  
739  
740  
741  
742  
743  
744  
745  
746  
747  
748  
749  
750  
751  
752  
753  
754  
755

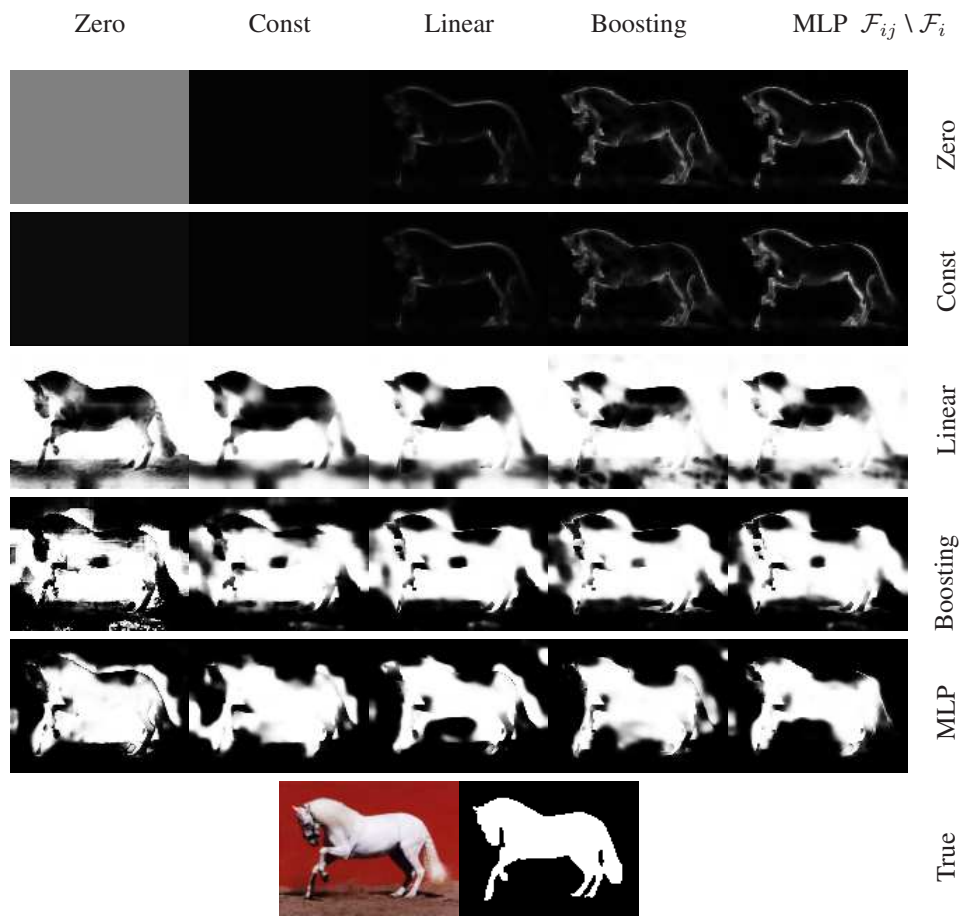

Figure 7: Example Predictions on the Horses Dataset

756  
757  
758  
759  
760  
761  
762  
763  
764  
765  
766  
767  
768  
769  
770  
771  
772  
773  
774  
775  
776  
777  
778  
779  
780  
781  
782  
783  
784  
785  
786  
787  
788  
789  
790  
791  
792  
793  
794  
795  
796  
797  
798  
799  
800  
801  
802  
803  
804  
805  
806  
807  
808  
809

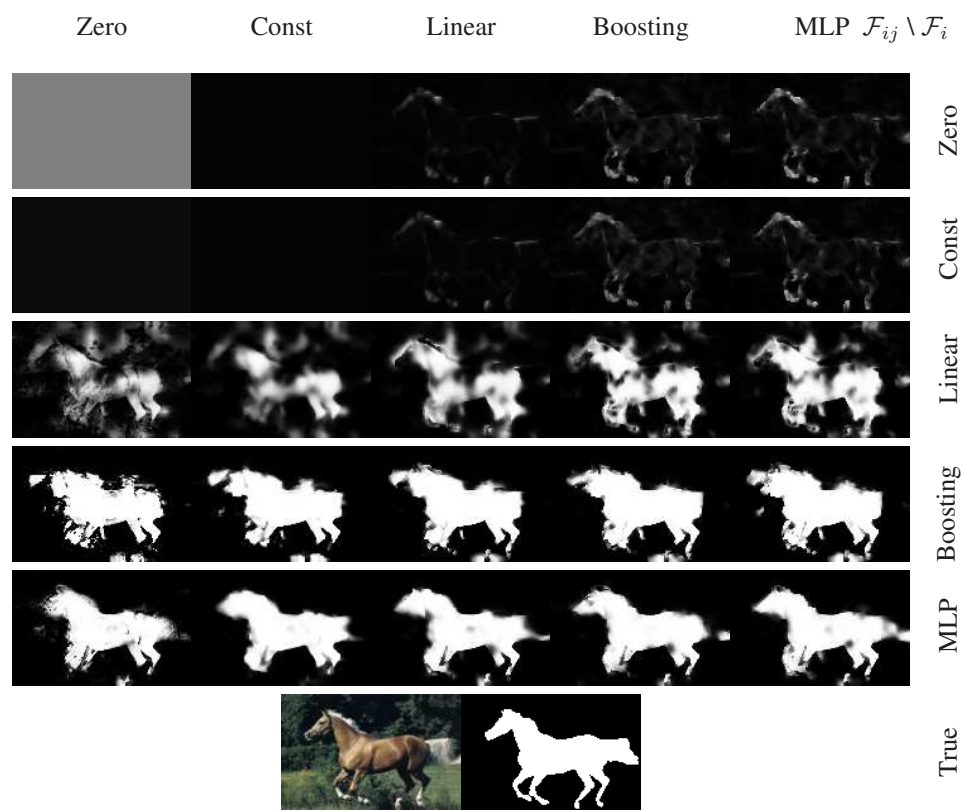

Figure 8: Example Predictions on the Horses Dataset

810  
811  
812  
813  
814  
815  
816  
817  
818  
819  
820  
821  
822  
823  
824  
825  
826  
827  
828  
829  
830  
831  
832  
833  
834  
835  
836  
837  
838  
839  
840  
841  
842  
843  
844  
845  
846  
847  
848  
849  
850  
851  
852  
853  
854  
855  
856  
857  
858  
859  
860  
861  
862  
863

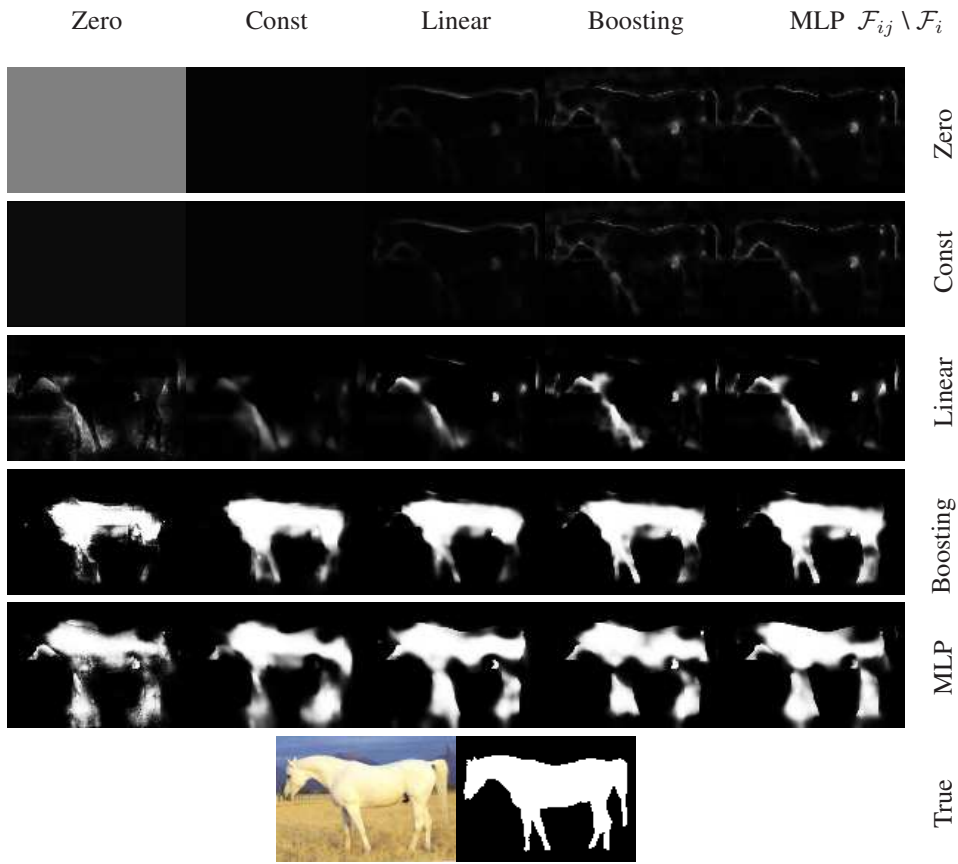

Figure 9: Example Predictions on the Horses Dataset

864  
865  
866  
867  
868  
869  
870  
871  
872  
873  
874  
875  
876  
877  
878  
879  
880  
881  
882  
883  
884  
885  
886  
887  
888  
889  
890  
891  
892  
893  
894  
895  
896  
897  
898  
899  
900  
901  
902  
903  
904  
905  
906  
907  
908  
909  
910  
911  
912  
913  
914  
915  
916  
917

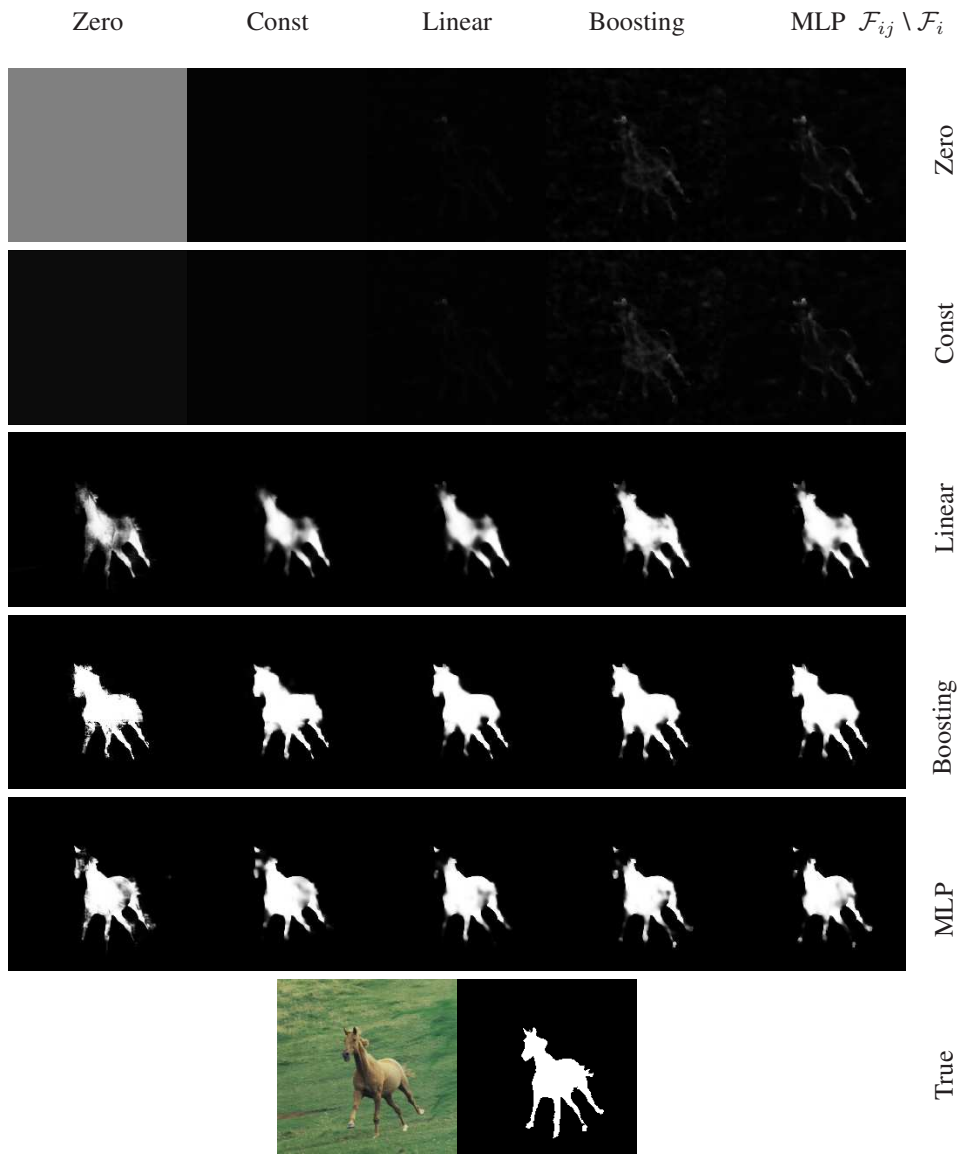

Figure 10: Example Predictions on the Horses Dataset

918  
919  
920  
921  
922  
923  
924  
925  
926  
927  
928  
929  
930  
931  
932  
933  
934  
935  
936  
937  
938  
939  
940  
941  
942  
943  
944  
945  
946  
947  
948  
949  
950  
951  
952  
953  
954  
955  
956  
957  
958  
959  
960  
961  
962  
963  
964  
965  
966  
967  
968  
969  
970  
971

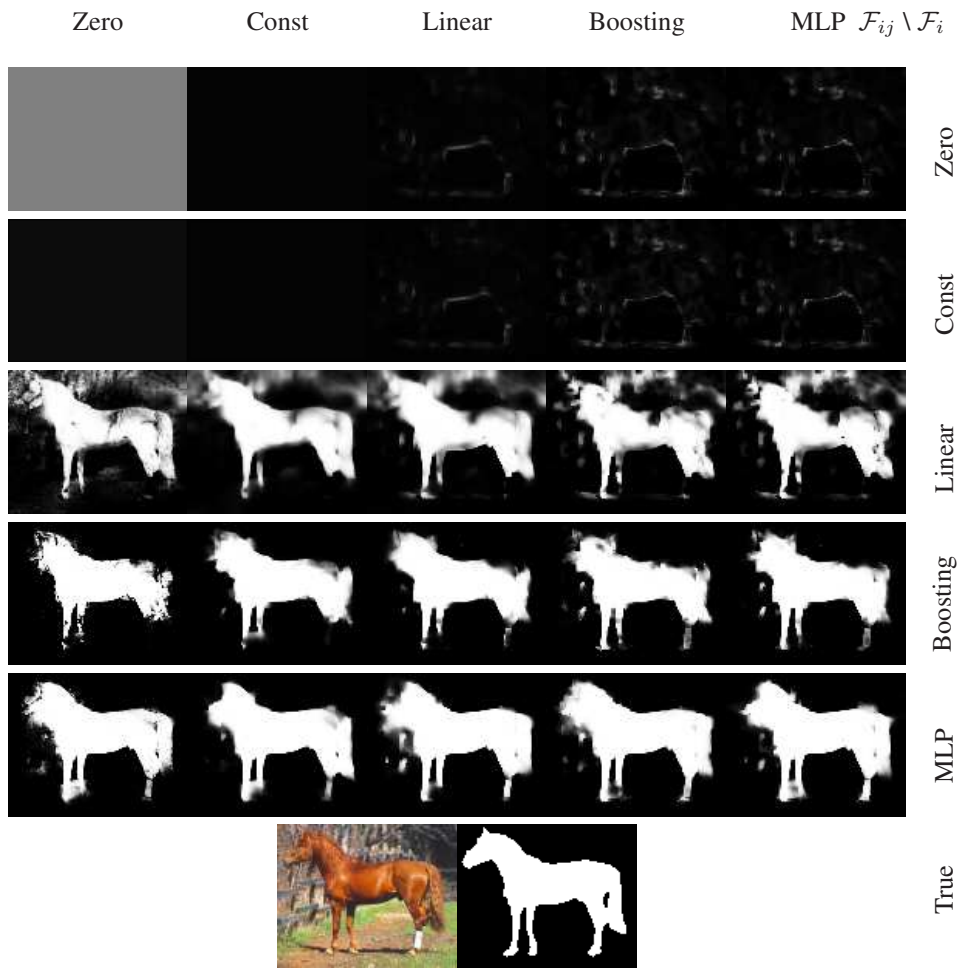

Figure 11: Example Predictions on the Horses Dataset

972  
 973  
 974  
 975  
 976  
 977  
 978  
 979  
 980  
 981  
 982  
 983  
 984  
 985  
 986  
 987  
 988  
 989  
 990  
 991  
 992  
 993  
 994  
 995  
 996  
 997  
 998  
 999  
 1000  
 1001  
 1002  
 1003  
 1004  
 1005  
 1006  
 1007  
 1008  
 1009  
 1010  
 1011  
 1012  
 1013  
 1014  
 1015  
 1016  
 1017  
 1018  
 1019  
 1020  
 1021  
 1022  
 1023  
 1024  
 1025

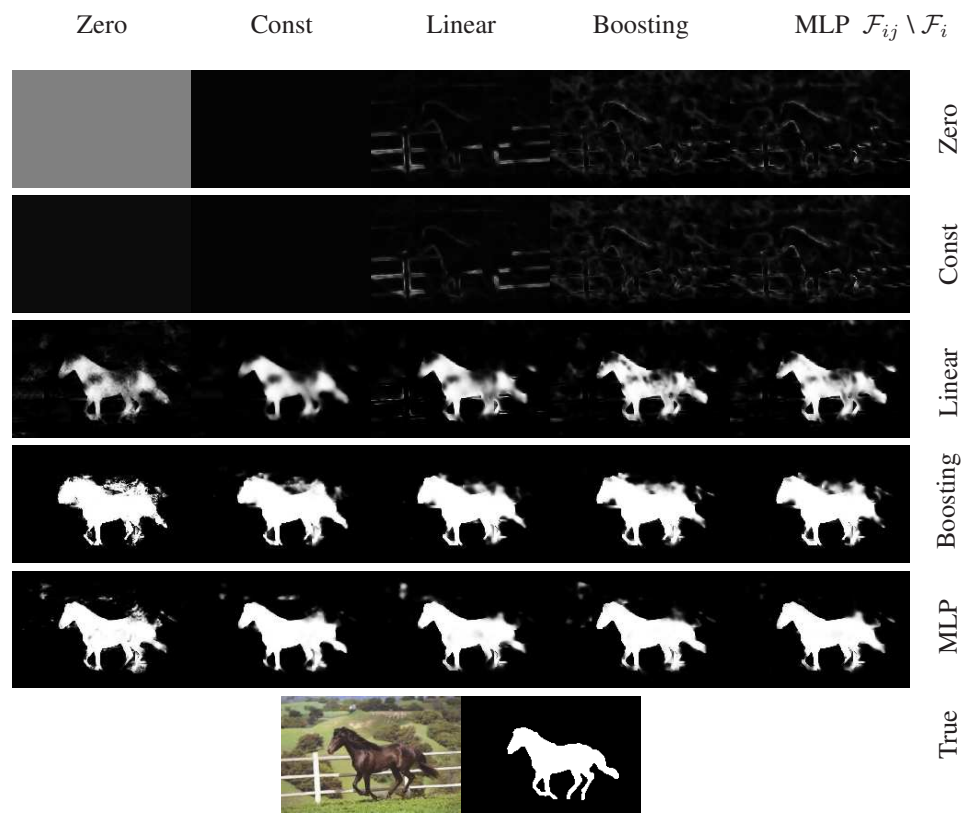

Figure 12: Example Predictions on the Horses Dataset
